# Supplementary material for: Hybrid divide-and-conquer approach for tree search algorithms
Source: arXiv:2007.07040 source file (2023-03-20)
Supplement: Supplementary file 1 [file appendix-walk-operator.tex]

\section{Implementing the walk operator}
\label{sub:implement-walk}

In this section, we describe step by step an implementation of the walk operator $W$, for $k$-SAT solving backtracking algorithms. As $W$ is the operator $R_BR_A$, we focus on the implementation of the subroutines $R_A$ and $R_B$. Let $x$ be a partial assignment of the formula (i.e. a vertex in our search tree).

For now, we assume that we are given access to an unitary $V_A$ which computes the two neighbours $x_1$ and $x_2$ of the vertex $x$. 
\[
V_A: \ket{x}\ket{0}\ket{0} \mapsto \ket{x}\ket{x_1}\ket{x_2}
\]
In order to implement this unitary, we first implement a routine which determines the next variable which will be guessed, and exploit that routine to obtain two unitaries $V_1\ket{x}\ket{0}\ket{y} =\ket{x}\ket{y_1}\ket{y}$ and 
$V_2\ket{x}\ket{y}\ket{0} =\ket{x}\ket{y}\ket{y_2}$. Those unitaries are formally implemented in Appendix~\ref{sub:implement-unit} (for the unit rule) and Appendix~\ref{sub:implement-pure} (for the pure literal rule).

Moreover, we assume that we are given access to an unitary $V_C$ which, given three vertices outputs their sum, i.e.
\[
V_C \ket{x}\ket{y}\ket{z} = \frac{1}{\sqrt{3}} \ket{x}\ket{y}\ket{z} \left(\ket{x}+\ket{y}+\ket{z} \right)
\]
The unitary $V_C$ is formally implemented in Appendix~\ref{sub:implement-combining}.

Finally, we make use of the unitary $V_\text{leaf}$ which checks whether all the variables in $x$ have been assigned (i.e. $x$ is a leaf of the search tree). This is an unitary such that $V_\text{leaf}\ket{x}\ket{0} = \ket{x}\ket{b}$, where $b$ is a Boolean value equal to $1$ if and only if $x$ is a leaf. Similarly, we make use of the unitary $V_\text{marked}$ such that $V_\text{marked}\ket{x}\ket{0}=\ket{x}\ket{b}$, where $b$ is a Boolean value equal to $1$ if and only if $x$ is a satisfying assignment.

Now, the operator $R_A$ can be implemented by checking whether the vertex $x$ is marked, and otherwise applying $U_A\left(\text{Id} - \ket{0}\bra{0}\right)U^\dagger_A$, where $U_A = \bigoplus_{x \in A} U_A^x$ is the unitary which computes the state $\ket{\varphi_x}$, i.e.~
\[
U_A\ket{x}\ket{0}=\ket{x}U_A^x\ket{0}=\ket{x}\ket{\varphi_x}
\] 

Recall the definitions of the states 
\[
\ket{\varphi_x} = \frac{1}{\sqrt{d_x}} \left(\ket{x} + \sum_{x \to y} \ket{y}\right)
\] 
for $x \neq r$, and the state 
\[
\ket{\varphi_r} = \frac{1}{\sqrt{d_r}n + 1} \left(\ket{r} + \sqrt{n} \cdot \sum_{r \to y} \ket{y}\right).
\]

In order to implement $R_A$, we implement the diffusion operator $D_x$ as an unitary $U_A^x$ such that $U_A^x\ket{0}=\ket{\varphi_x}$. When $x$ is a leaf, $\ket{\varphi_x}=\ket{x}$ and $U_A^x$ simply copies $\ket{x}$. When $x$ is not a leaf, $U_A^x$ is implemented by the unitary $V^\dagger_A V_C V_A$, where the unitaries $V_A$ and $V_C$ are respectively implemented in Section~\ref{sub:implement-unit} and Section~\ref{sub:implement-combining}. We use the unitary $V_\text{leaf}$ (respectively $V_\text{marked}$) to control whether $x$ is a leaf (respectively a satisfying assignment).% see Section~\ref{sub:formula-evaluation} for an explanation of the implementation of formula evaluation.

The operator $R_B$ is implemented in a similar fashion to $R_A$, assuming that we have access to an unitary $V_\text{root}$ which checks whether $x = r$. Observing that the root is associated to the all-undetermined satisfying assignment $\star^n$. Such an unitary can easily be implemented by a succession of CNOT gates followed by a Pauli-X gate, controlled on each variable being equal to $\star$.

Recall that in the search trees generated by backtracking algorithms which fit within the framework of Theorem~\ref{th:metatheorem} are such that every vertex has either $0$ children (and is therefore a leaf), $1$ child (when a reduction rule is applied), or $2$ children (when a variable is guessed). However, a single-child version of $V_A$ can easily be implemented, as explained in Appendix~\ref{sub:implement-combining}.

Now, let us analyse the cost of the implementation of the walk operator $W$. Firstly, we observe that, having access to the unitary $R_A$ and $R_B$, implementing $W$ can be done with an ancilla qubit which checks whether the vertex $x$ that we are considering is odd or even.

To be more specific, in previous implementations of quantum backtracking~\cite{qbacktracking,campbell-qCSP,practical-qbacktracking}, a depth counter is maintained to determine the parity of the depth at which the vertex $x$ is. We forgo of such a register by observing that each variable assignment takes us one level deeper into the tree, and therefore the depth at which $x$ is at is given is defined by the number of variables which have already been assigned a value. Therefore, to check the parity of the depth, it suffices to use one ancilla qubit, and check each qutrit $x_i$ of the register $\ket{x}$, flipping the ancilla qubit every time $x_i \neq *$.

It follows that the cost of implementing the quantum walk operator $W$ can be bounded as follows.
\[\cost{W} \leq \text{max}(\cost{R_A},\cost{R_B}) +1.\] 

As we have just seen, the operators $R_A$ and $R_B$ have very similar implementations. Now, under our current implementation ,
\begin{align*}
\cost{R_A} &\leq \cost{U_A} +1 \\
	&\leq \log_2(3)(n+1) + \cost{V_A} + \cost{V_C} + 2
\end{align*}
where $\cost{V_A} \in O(\log(n))$ (see Section~\ref{sub:implement-unit}) and  $\cost{V_C} \leq 5\log_2(3)$ (see Section~\ref{sub:implement-combining}).
% so that $W$ can be implemented using at most $\log_2(3)(n+6) + O(\log(n))$.
Thus, we deduce the following theorem.

\begin{theorem}
\label{thm:implement-walk}
Assuming access to the unitaries $V_A$, $V_C$, $V_\text{leaf}$, $V_\text{marked}$ and $V_\text{root}$, one can implement the walk operator using at most $\log_2(3)n+w$ qubits, with $w \in O(\log(n))$.
\end{theorem}

\subsection{Implementing the unit clause rule}
\label{sub:implement-unit}

In order to determine the next vertices in the search tree according to the unit rule, one needs to determine whether there exists an unit clause (i.e. a clause $C=\{l\}$ with only one literal $l$), given a partial assignment of the formula that we are considering. Whenever a unit clause is found, no branching occurs and the literal is simply set to true.

In order to implement this process, we need two operations:
\begin{itemize}
 \item An operation $V^{(i)}_\text{unit}$ which checks whether the $i$-th clause is an unit clause.
 \item An operation $V_\text{next}$ which outputs the next partial assignment.
\end{itemize}

\begin{figure}
\mbox{
 \Qcircuit @C=1em @R=.7em {
  \lstick{\ket{0}} & \qw & \qw & \qw & \multigate{1}{\text{IsUnit}_i}  & \qw & \ctrl{3} & \qw & \qw & \qw \\
  \lstick{\ket{x}} & /^n \qw & \multigate{1}{\mathcal{C}_i} & \qw & \ghost{\text{IsUnit}_i} & \qw & \qw & \qw & \multigate{1}{\mathcal{C}_i^\dagger} & \qw\\
  \lstick{\ket{0}} & \qw  & \ghost{\mathcal{C}_i}  & \qw & \ctrl{-1} & \qw & \ctrl{1} & \qw & \ghost{\mathcal{C}_i^\dagger} & \qw\\
  \lstick{\ket{0}} & \qw & \qw & \qw & \qw & \qw & \targ & \qw & \qw & \qw
 }
 }
\caption{\label{fig:unit-clause-i} Checks whether $C_i$ is an unit clause}
\end{figure}

\begin{figure}
\mbox{
 \Qcircuit @C=1em @R=.7em {
  \lstick{\ket{0}_\text{sign}} & \qw & \qw & \qw & \multigate{2}{\text{Check}_{j,i}}  & \qw & \ctrl{3} & \ctrlo{3} & \qw  & \qw \\
  \lstick{\ket{0}_\text{unit?}} & \qw & \qw & \qw & \ghost{\text{Check}_{j,i}}  & \qw & \ctrl{3} & \ctrl{4} & \qw & \qw \\
  \lstick{\ket{x}} & /^n \qw & \multigate{1}{\mathcal{C}_j} & \qw & \ghost{\text{Check}_{j,i}} & \qw & \qw & \qw & \multigate{1}{\mathcal{C}_j^\dagger} & \qw\\
  \lstick{\ket{0}} & \qw  & \ghost{\mathcal{C}_j}  & \qw & \ctrl{-1} & \qw & \qw & \qw & \ghost{\mathcal{C}_j^\dagger} & \qw\\
  \lstick{\ket{c_+}} & \qw & \qw & \qw & \qw & \qw & \gate{inc} & \qw & \qw & \qw  \\
  \lstick{\ket{c_-}} & \qw & \qw & \qw & \qw & \qw & \qw & \gate{inc} & \qw & \qw \\
 }
 }
\caption{\label{fig:pure-sub} Subroutine of $V_\text{pure}$}
\end{figure}

\begin{figure*}
\mbox{
 \Qcircuit @C=1em @R=.7em {
 & & & & & & & & & \mbox{~~~~~\textbf{U}}\\
  \lstick{\ket{x}} & /^n \qw & \multigate{2}{V_\text{unit}^1} & \qw & \qw & \cdots & & \qw & \multigate{2}{V_\text{unit}^L} & \qw & \qw & \qw & \multigate{3}{U^\dagger} & \qw\\
  \lstick{\ket{0}} & \qw  & \ghost{V_\text{unit}^1}  & \ctrl{2} & \qw & \cdots & & \qw & \ghost{V_\text{unit}^L} & \ctrl{2} & \ctrl{3} & \qw & \ghost{U^\dagger} & \qw\\
  \lstick{\ket{0}} & \qw & \ghost{V_\text{unit}^1} & \qw & \qw & \cdots & & \qw & \ghost{V_\text{unit}^L} & \qw & \qw  & \ctrl{3} & \ghost{U^\dagger} & \qw\\
  \lstick{\ket{0}} & \qw & \ctrlo{-1} & \gate{inc} & \qw & \cdots & & \qw & \ctrlo{-1} & \gate{inc} \gategroup{1}{2}{5}{10}{.7em}{--} & \qw &\qw & \qw & \qw \\
  \lstick{\ket{0}} & \qw & \qw & \qw & \qw & \qw & \qw & \qw & \qw & \qw & \targ & \qw & \qw & \qw\\
  \lstick{\ket{0}} & \qw & \qw & \qw & \qw & \qw & \qw &\qw &\qw &\qw &\qw &\targ &\qw &\qw
 }
 }
\caption{\label{fig:unit-clause} Checks whether there is an unit clause}
\end{figure*}

We define an operation $V^{(i)}_\text{unit}$ which checks whether the $i$-th clause $C_i$ is an unit clause. The operator $V^{(i)}_\text{unit}$ can be implemented efficiently and reversibly, using the subroutine describe in Figure~\ref{fig:unit-clause-i}, and if an unit clause is found, queries to the index and the sign of the variable which is part of the unit clause. Note that the unitary $\mathcal{C}_i$ evaluates the clause $C_i$ for $x$, and the unitary $\text{IsUnit}_i$ checks whether $k-1$ variables of the clause $C_i$ have been assigned a value: it is implemented with a counter from $0$ till $k$, with an incrementation controlled on variables having a value different from $\ast$.

Then, each clause $C_i$ is associated to the unitary $V^{(i)}_\text{unit}:\ket{x}\ket{0}\ket{0}\mapsto\ket{x}\ket{j}\ket{s}$. In order to apply the unit rule, we apply $V^{(i)}_\text{unit}$ to each clause $C_i$ in the formula studied, and stop whenever we find an unit clause (i.e. whenever $V^{(i)}_\text{unit}$ outputs $\ket{x}\ket{j}\ket{1}$), see Figure~\ref{fig:unit-clause}.

Note that, to go through all the $L$ clauses of a formula, we need a clause counter which is implemented using $\lceil\log(L)\rceil$ ancilla bits, with $\lceil\log(L)\rceil < \lceil k \cdot \log_2(n) \rceil$ since a k-SAT formula has at most ${k \choose 2n} \leq \frac{(2n)^k}{k!} < \frac{4}{3} n^k$ clauses.

If an unit clause is found, its variable is assigned a value. If no unit clause was found, the unit rule is not applied and the unitaries $V_1$ and $V_2$ can easily be obtained from an unitary
$
V_\text{next}: \ket{x}\ket{0}\ket{j}\ket{b} \mapsto \ket{x}\ket{x'}\ket{j}\ket{b}
$
where $x'$ is defined as the partial assignement $x$ with $x_j$ set to $b$. Such an unitary is implemented by copying $x$ to the output register, then checking for the $j$-th index, assigning the value $b$ to the one whose index is $j$.

If the unit rule is not applied, we obtain $V_1$ (resp. $V_2$) by applying $V_\text{next}$ with $\ket{b}=\ket{0}$ (resp. $\ket{b}=1$), so that given $\ket{x}\ket{0}\ket{j}\ket{0}$, $V_1$ (resp. $V_2$) outputs $\ket{x}\ket{x[x_j=0]}\ket{j}\ket{0}$ (resp. $\ket{x}\ket{x[x_j=1]}\ket{j}\ket{1}$), and therefore $V_A:\ket{x}\ket{0}\ket{0}\mapsto\ket{x}\ket{x[x_j=0]}\ket{x[x_j=1]}$.

If the unit rule is applied, the current vertex only has one neighbour, given by $V_1$ which is obtained by applying $V_\text{next}$ with $\ket{b}=\ket{0}$ if the formula contains the $\{x_j\}$, and $\ket{b}=\ket{1}$ if the formula contains the $\{\overline{x}_j\}$.

%Finally, note that the time complexity of each extraction operation is proportional to $nk$. The extraction routine runs the shifting routine $nk$ times, and therefore take a time proportional to $n^2k^2$. Since our implementation $\text{Contains}_K$ extracts each variable of a clause, it takes $n^2k^3$. Therefore, our implementation of the unit rule takes a time proportional to $n^2k^3L$.

\subsection{Implementing the pure literal rule}
\label{sub:implement-pure}

The pure literal rule eliminates variables $x_i$ which only appear as the literal $x_i$ or only appear as the literal $\overline{x_i}$. In which case, the variable is set to the value which makes the literal true, eliminating all the clauses which contains it in the process. Classically, it is a convenient way to reduce the number of clauses manipulated by the backtracking algorithm considered. However, the quantum backtracking implementation that we present in this paper is not concerned with formula rewriting. If a pure literal exists, we only need to know the index of its variable, and the value which has to be assigned. Therefore, it suffices to implement the following operator:
\[
V_\text{pure}:\ket{x}\ket{0}_\text{index}\ket{0}_\text{sign} \mapsto 
\ket{x}\ket{i}_\text{index}\ket{s}_\text{sign}
\]
where $i$ is the index of the variable $x_i$ which is a positive ($s=0$) or negative ($s=1$) pure literal ($i=0$ if it does not exists), or the index of the last variable checked if no pure literal was found ($b=0$). The implementation of the unitary $V_\text{pure}$ is quite similar to the implementation of the unit rule. For each variable $x_i$, if no pure literal was found (that is, the index output register is still zero), we maintain two clause counters to count the number of (unsatisfied) clauses in which $x_i$ and $\bar{x}_i$ respectively appear, as described in Figure~\ref{fig:pure-sub}. Using a Toffoli gate, we determine whether only one of the counter is equal to $0$, and if it is the case, we copy the index and sign of $x_i$ in the output register. Finally, we uncompute the ancillas by applying the inverse of the circuit so far (as we did for the unit rule, see Figure~\ref{fig:unit-clause}). This procedure is implemented using $2\lceil \log_2(L)\rceil + O(1)$ ancillas. 

As in the implementation of the unit rule (see~Appendix~\ref{sub:implement-unit}), we use $V_\text{next}$ to compute the next partial assignment.

\subsection{Combining vertices efficiently}
\label{sub:implement-combining}

In what follows, we implement the unitary which generates the state which encodes the sum of three vertices, with $n$ ancilla trits. This logarithmic overhead comes from the efficient encoding of the set of variables. In detail, we implement the following unitary
\begin{align*}
&V_C \ket{x_0}\ket{x_1}\ket{x_2}\ket{0}_\text{sum}\ket{0}_\text{anc}\\
&= \frac{1}{\sqrt{3}} \ket{x_0}\ket{x_1}\ket{x_2} \left(\ket{x_0}+\ket{x_1}+\ket{x_2} \right)_\text{sum}\ket{0}_\text{anc}
\end{align*}
as follows.

We first rotate the ancilla trit to $\frac{1}{\sqrt{3}} \left(\ket{0}+\ket{1}+\ket{2}\right)$ then copy each vertex in one of the ancilla trits which stores the sum, resulting in the state
\begin{equation}
\label{eq:sum-before-3QFT}
\frac{1}{\sqrt{3}} \sum_{0 \leq i \leq 2} \left(\ket{x_0}\ket{x_1}\ket{x_2}\ket{x_i}\ket{i}\right)
\end{equation}

Then, consider the Quantum Fourier Transform 3QFT which sends the basis qutrit state to the superposition
\begin{equation}
\label{eq:3QFT}
\sum_{0 \leq j \leq 2} \ket{j}\bra{\omega_j}
\end{equation}
where $\ket{\omega_j}$ is the $j$-th column of the matrix of the quantum fourier transform.

Now, we apply 3QFT and uncompute the phases it introduces, we obtain the following state
\begin{equation}
\frac{1}{\sqrt{3}} \ket{x_0}\ket{x_1}\ket{x_2} \left(\sum_{0 \leq i \leq 2} \ket{x_i}\right)_\text{sum} \sum_{0 \leq j \leq 2} \ket{j}_\text{anc}
\end{equation}
We finally apply the inverse rotation to the ancilla trit register, resulting in the state
\begin{equation}
\frac{1}{\sqrt{3}} \ket{x_0}\ket{x_1}\ket{x_2} \left(\sum_{0 \leq i \leq 2} \ket{x_i}\right)_\text{sum}\ket{0}_\text{anc}
\end{equation}

It remains to explain how one can uncompute the phases. Applying the 3QFT of Equation~\ref{eq:3QFT} to the state in Equation~\ref{eq:sum-before-3QFT} results in the following state
\begin{equation}
\label{eq:state-with-phases}
\frac{1}{\sqrt{3}}  \sum_{j=0}^2 \ket{x_0}\ket{x_1}\ket{x_2} 
\left(\sum_{0 \leq i \leq 2} \left\langle \phi_j \mid j \right\rangle \ket{x_i}\right)_\text{sum} \ket{j}_\text{anc}
\end{equation}
Therefore, we need an unitary which transforms the state in Equation~\ref{eq:state-with-phases} in the following state
\[
\frac{1}{\sqrt{3}}  \sum_{j=0}^2 \ket{x_0}\ket{x_1}\ket{x_2} 
\left(\sum_{0 \leq i \leq 2} e^{i \theta_i} \left\langle \phi_j \mid j \right\rangle \ket{x_i}\right)_\text{sum} \ket{j}_\text{anc}
\]
where the $\theta_i$'s are phases which cancel out $\left\langle \phi_j \mid j \right\rangle$.

For each register $i$, we add a phase $\theta_i$ by applying the phase shift $P_{\theta_i} = (\mathrm{1} - \ket{i}\bra{i}) + e^{i \theta_i} \ket{i}\bra{i}$ on the register $i$.

Overall, the cost of the routine is constant, i.e. $\cost{V_C} \leq \lceil 5\log_2(3) \rceil=8$. The time complexity is linear in $n$.

For vertices which only have one children in the search tree, we can similarly implement the unitary which generates the state which encodes the sum of a vertex $x$ and its unique child $y$. In detail, we implement the unitary 
\[
V_C \ket{x}\ket{y}\ket{0}_\text{sum}\ket{0}_\text{anc} = \frac{1}{\sqrt{2}} \ket{x}\ket{y} \left(\ket{x}+\ket{y} \right)_\text{sum}\ket{0}_\text{anc}
\]
applying Hadamard gates to the ancilla register, instead of 3QFTs.

\section{Quantum tree size estimation}
\label{sec:quantum-tree-size-estimation}
One drawback of Montanaro's quantum backtracking is that the runtime depends on the estimate of the size of the search tree (which is a parameter of the algorithm), and not on the size of the subtree that the classical backtracking algorithm explores. 

The efficiency of a classical backtracking algorithm relies on its ability to explore the most promising branches first, which means than in practice, the algorithm may find a marked vertex after exploring $T'$ vertices, where $T' \ll T$. Using a quantum tree size estimation subroutine to estimate the size of the subtree explored by the classical backtracking algorithm, there is an improvement on the original quantum backtracking algorithms which covers this $T' \ll T$ case \cite{ambainis-kokainis}.

\begin{theorem}
\label{th:ambainis}
Consider a classical backtracking algorithm $\mathcal A$ which generates a search tree $\mathcal T$. There is a quantum algorithm which outputs $1$ with high probability if $\mathcal T$ contains a marked vertex and $0$ if it doesn't, with query complexity $O(n^{\frac{3}{2}}\sqrt{T'})$         
where $T'$ is the number of vertices actually explored by $\mathcal{A}$.
\end{theorem}

The overall algorithm generates subtrees which contain the first $2^i$ vertices explored by the classical backtracking algorithm, increasing $i$ until a marked vertex is found, or the whole search tree is considered. It is on each subtree containing the first $2^i$ vertices that we run the quantum backtracking algorithm.

Note that quantum backtracking with tree size estimation is only considered when $T' \ll T$. Because this algorithm is less performant than the original when $T'$ is close to $T$, one can just switch to Montanaro's algorithm whenever the complexity of the generation of the path exceeds the complexity of the original quantum backtracking.

The main component of this variant of Montanaro's quantum backtracking, are quantum backtracking itself, and the quantum tree size estimation algorithm, which is a variant of quantum backtracking with the same space complexity. Therefore it is sufficient to prove that quantum backtracking can be implemented efficiently in order to benefit from the speedup provided by Theorem~\ref{th:ambainis} in the hybrid framework.

%Performing this algorithm up to precision $\varepsilon$ requires to perform quantum phase estimation to a $t$-bit precision, where $t=\left\lceil\frac{9}{4}\ln\left(\frac{2}{\varepsilon'}\right)\right\rceil$, where %$C=\frac{4}{9}$, and 
%$\varepsilon'=\left\lceil\frac{\varepsilon}{\lceil2\log(T)\rceil}\right\rceil$.
